# Supplementary material for: Simplifying Complex Observation Models in Continuous POMDP Planning with Probabilistic Guarantees and Practice
Source: arXiv:2311.07745 source file (2025-05-24)
Supplement: Supplementary file 1 [file technical_appendix.tex]

%File: appendices.tex
\documentclass[letterpaper]{article} % DO NOT CHANGE THIS
\usepackage{aaai24}  % DO NOT CHANGE THIS
\usepackage{times}  % DO NOT CHANGE THIS
\usepackage{helvet}  % DO NOT CHANGE THIS
\usepackage{courier}  % DO NOT CHANGE THIS
\usepackage[hyphens]{url}  % DO NOT CHANGE THIS
\usepackage{graphicx} % DO NOT CHANGE THIS
\urlstyle{rm} % DO NOT CHANGE THIS
  % DO NOT CHANGE THIS
\usepackage{natbib}  % DO NOT CHANGE THIS AND DO NOT ADD ANY OPTIONS TO IT
\usepackage{caption} % DO NOT CHANGE THIS AND DO NOT ADD ANY OPTIONS TO IT
\frenchspacing  % DO NOT CHANGE THIS
\setlength{\pdfpagewidth}{8.5in} % DO NOT CHANGE THIS
\setlength{\pdfpageheight}{11in} % DO NOT CHANGE THIS
%
% These are recommended to typeset algorithms but not required. See the subsubsection on algorithms. Remove them if you don't have algorithms in your paper.
\usepackage{algorithm}
\usepackage[noend]{algorithmic}
% \usepackage{algpseudocode}

%
% These are are recommended to typeset listings but not required. See the subsubsection on listing. Remove this block if you don't have listings in your paper.
\usepackage{newfloat}
\usepackage{listings}
\DeclareCaptionStyle{ruled}{labelfont=normalfont,labelsep=colon,strut=off} % DO NOT CHANGE THIS
\lstset{%
	basicstyle={\footnotesize\ttfamily},% footnotesize acceptable for monospace
	numbers=left,numberstyle=\footnotesize,xleftmargin=2em,% show line numbers, remove this entire line if you don't want the numbers.
	aboveskip=0pt,belowskip=0pt,%
	showstringspaces=false,tabsize=2,breaklines=true}
\floatstyle{ruled}
\newfloat{listing}{tb}{lst}{}
\floatname{listing}{Listing}
%
% Keep the \pdfinfo as shown here. There's no need
% for you to add the /Title and /Author tags.
\pdfinfo{
/TemplateVersion (2024.1)
}

\usepackage{amsmath}
\usepackage{amssymb}
\usepackage{xspace}
\usepackage{amsthm}
\usepackage{subcaption}
\usepackage{multirow}
\usepackage{booktabs}
\usepackage{xcolor}
\usepackage{import}
\usepackage{enumitem}
\usepackage{cancel}
\usepackage{mathtools}
\usepackage{tabularx}
\allowdisplaybreaks  

%%% END OUR PACKAGES %%%%%%%

%%% BEGIN OUR COMMANDS %%%%%

 %\mathsf{P}}

\newcommand{\CondCurlyBrackets}[1]{\expandafter\ifx\expandafter\relax\detokenize{#1}\relax\else\left(#1\right)\fi}
\newcommand{\CondRectBrackets}[1]{\expandafter\ifx\expandafter\relax\detokenize{#1}\relax\else[#1]\fi}
\newcommand{\CondRectBracketsHigh}[1]{\expandafter\ifx\expandafter\relax\detokenize{#1}\relax\else\left[#1\right]\fi}
\newcommand{\CondColon}[1]{\expandafter\ifx\expandafter\relax\detokenize{#1}\relax\else:{#1}\fi}

  % Delta z
  % Delta z approximate 
  % m importance sampling

  % Policy at time i

\makeatletter
\newtheorem*{rep@theorem}{\rep@title}
\newcommand{\newreptheorem}[2]{%
\newenvironment{rep#1}[1]{%
 \def\rep@title{#2 \ref{##1}}%
 \begin{rep@theorem}}%
 {\end{rep@theorem}}}
\makeatother

\theoremstyle{plain}

\theoremstyle{plain}

\theoremstyle{plain}

\providecommand{\theoremrptname}{Theorem}
\providecommand{\lemmarptname}{Lemma}
\providecommand{\corollaryrptname}{Corollary}

%%%% Declaration of theorem envs with thmtools
% \declaretheorem{theorem}
% \declaretheorem{lemma}
% \declaretheorem{corollary}
%%%% With explicit ref names
% \declaretheorem[name=Theorem, refname={theorem,theorems}, Refname={Theorem,Theorems}]{theorem}
% \declaretheorem[name=Lemma, refname={lemma,lemmas}, Refname={Lemma,Lemmas}]{lemma}
% \declaretheorem[name=Corollary, refname={corollary,corollaries}, Refname={Corollary,Corollaries}]{corollary}

%%% END OUR COMMANDS %%%%%%%

\setcounter{secnumdepth}{2} %May be changed to 1 or 2 if section numbers are desired.

% The file aaai24.sty is the style file for AAAI Press
% proceedings, working notes, and technical reports.
%

% Title

% Your title must be in mixed case, not sentence case.
% That means all verbs (including short verbs like be, is, using,and go),
% nouns, adverbs, adjectives should be capitalized, including both words in hyphenated terms, while
% articles, conjunctions, and prepositions are lower case unless they
% directly follow a colon or long dash
\iffalse
\title{AAAI Press Anonymous Submission\\Instructions for Authors Using \LaTeX{}}
\author{
    %Authors
    % All authors must be in the same font size and format.
    Written by AAAI Press Staff\textsuperscript{\rm 1}\thanks{With help from the AAAI Publications Committee.}\\
    AAAI Style Contributions by Pater Patel Schneider,
    Sunil Issar,\\
    J. Scott Penberthy,
    George Ferguson,
    Hans Guesgen,
    Francisco Cruz\equalcontrib,
    Marc Pujol-Gonzalez\equalcontrib
}
\affiliations{
    %Afiliations
    \textsuperscript{\rm 1}Association for the Advancement of Artificial Intelligence\\
    % If you have multiple authors and multiple affiliations
    % use superscripts in text and roman font to identify them.
    % For example,

    % Sunil Issar\textsuperscript{\rm 2},
    % J. Scott Penberthy\textsuperscript{\rm 3},
    % George Ferguson\textsuperscript{\rm 4},
    % Hans Guesgen\textsuperscript{\rm 5}
    % Note that the comma should be placed after the superscript

    1900 Embarcadero Road, Suite 101\\
    Palo Alto, California 94303-3310 USA\\
    % email address must be in roman text type, not monospace or sans serif
    proceedings-questions@aaai.org
%
% See more examples next
}
\fi

%Example, Single Author, ->> remove \iffalse,\fi and place them surrounding AAAI title to use it
\iffalse
\title{My Publication Title --- Single Author}
\author {
    Author Name
}
\affiliations{
    Affiliation\\
    Affiliation Line 2\\
    name@example.com
}
\fi

%Example, Multiple Authors, ->> remove \iffalse,\fi and place them surrounding AAAI title to use it
\title{Simplifying Complex Observation Models in Continuous POMDP Planning with Probabilistic Guarantees and Practice - Supplementary Material}
\author {
    % Authors
    Idan Lev-Yehudi\textsuperscript{\rm 1},
    Moran Barenboim\textsuperscript{\rm 1},
    Vadim Indelman\textsuperscript{\rm 2}
}
\affiliations {
    % Affiliations
    \textsuperscript{\rm 1}Technion Autonomous Systems Program (TASP), Technion - Israel Institute of Technology, Haifa 32000, Israel\\
    \textsuperscript{\rm 2}Department of Aerospace Engineering, Technion - Israel Institute of Technology, Haifa 32000, Israel\\
    {moranbar, idanlev}@campus.technion.ac.il,
    vadim.indelman@technion.ac.il
}

\begin{document}

\maketitle

\appendix

\input{appendix_content.tex}

\bibliography{../refs}

\end{document}
